# Supplementary material for: Supervised Feature Selection with Neuron Evolution in Sparse Neural Networks
Source: arXiv:2303.07200 source file (2023-03-14)
Supplement: Supplementary file 1 [file results_supervised.tex]

\begin{table}[t]
    \centering
    \caption{Supervised feature selection comparison (classification accuracy (\%)) for different values of $K$ (number of selected features). Empty entries show that the corresponding experiments have exceeded the considered time limit (12 hours)} \label{tab:results_supervised_appendix} 
    \begin{scriptsize}
    
\scalebox{0.85}{
    \begin{tabular}{@{}c@{\hskip 0.04in}c@{\hskip 0.04in}c@{\hskip 0.04in}c@{\hskip 0.04in}c@{\hskip 0.04in}c@{\hskip 0.04in}c@{\hskip 0.04in}c@{\hskip 0.04in}}
        \toprule
         &  & \multicolumn{6}{c}{ \bt $K$}  \\
        \bt Dataset & \bt Method &\bt 25 &\bt 50 & \bt75 & \bt100 & \bt150 & \bt200  \\ \midrule

\multirow{3}{*}{coil20}&Baseline&\multicolumn{6}{c}{100.0}\\
\multicolumn{1}{c}{}&NeuroFS&\pmb{$96.2\pm0.8$}&$98.8\pm0.2$&$98.9\pm0.3$&$99.2\pm0.5$&\pmb{$100.0\pm0.0$}&$99.9\pm0.1$\\
\multicolumn{1}{c}{}&LassoNet&$90.9\pm1.7$&$97.2\pm1.5$&\pmb{$99.1\pm0.3$}&$99.5\pm0.3$&\pmb{$100.0\pm0.0$}&\pmb{$100.0\pm0.0$}\\
\multicolumn{1}{c}{}&Fisher\_score&$24.7\pm0.0$&$74.0\pm0.0$&$76.0\pm0.0$&$80.2\pm0.0$&$81.2\pm0.0$&$84.0\pm0.0$\\
\multicolumn{1}{c}{}&Ll\_L21&$72.6\pm0.0$&$71.5\pm0.0$&$75.7\pm0.0$&$75.7\pm0.0$&$76.4\pm0.0$&$79.2\pm0.0$\\
\multicolumn{1}{c}{}&CIFE&$50.7\pm0.0$&$59.4\pm0.0$&$63.2\pm0.0$&$67.7\pm0.0$&$71.9\pm0.0$&$72.2\pm0.0$\\
\multicolumn{1}{c}{}&ICAP&$94.4\pm0.0$&\pmb{$99.3\pm0.0$}&$99.0\pm0.0$&\pmb{$100.0\pm0.0$}&\pmb{$100.0\pm0.0$}&$99.3\pm0.0$\\
\multicolumn{1}{c}{}&RFS&$34.7\pm0.0$&$66.3\pm0.0$&$72.2\pm0.0$&$78.5\pm0.0$&$86.1\pm0.0$&$90.3\pm0.0$\\
\midrule

\multirow{3}{*}{MNIST}&Baseline&\multicolumn{6}{c}{97.9}\\
\multicolumn{1}{c}{}&NeuroFS&\pmb{$87.9\pm1.8$}&\pmb{$95.3\pm0.4$}&\pmb{$96.8\pm0.2$}&\pmb{$97.3\pm0.2$}&\pmb{$97.7\pm0.1$}&\pmb{$97.9\pm0.1$}\\
\multicolumn{1}{c}{}&LassoNet&$86.1\pm0.8$&$94.2\pm0.2$&$96.1\pm0.0$&$96.7\pm0.0$&$97.4\pm0.0$&$97.8\pm0.0$\\
\multicolumn{1}{c}{}&Fisher\_score&$74.4\pm0.0$&$81.9\pm0.0$&$87.1\pm0.0$&$90.7\pm0.0$&$93.1\pm0.0$&$94.5\pm0.0$\\
\multicolumn{1}{c}{}&Ll\_L21&$40.7\pm0.0$&$55.4\pm0.0$&$69.1\pm0.0$&$71.5\pm0.0$&$84.5\pm0.0$&$84.9\pm0.0$\\
\multicolumn{1}{c}{}&CIFE&$80.9\pm0.0$&$89.3\pm0.0$&$92.7\pm0.0$&$95.1\pm0.0$&$96.8\pm0.0$&$97.6\pm0.0$\\
\multicolumn{1}{c}{}&ICAP&$81.6\pm0.0$&$89.0\pm0.0$&$92.4\pm0.0$&$95.0\pm0.0$&$96.4\pm0.0$&$97.6\pm0.0$\\
\multicolumn{1}{c}{}&RFS&-&-&-&-&-&-\\
\midrule

\multirow{3}{*}{ \shortstack{Fashion-\\MNIST} }&Baseline&\multicolumn{6}{c}{88.3}\\
\multicolumn{1}{c}{}&NeuroFS&\pmb{$79.4\pm1.0$}&\pmb{$83.8\pm0.6$}&\pmb{$85.7\pm0.3$}&\pmb{$86.6\pm0.2$}&\pmb{$87.2\pm0.2$}&\pmb{$87.5\pm0.2$}\\
\multicolumn{1}{c}{}&LassoNet&$79.0\pm0.2$&$82.7\pm0.2$&$84.0\pm0.1$&$84.9\pm0.3$&$86.1\pm0.2$&$86.7\pm0.0$\\
\multicolumn{1}{c}{}&Fisher\_score&$53.1\pm0.0$&$67.8\pm0.0$&$74.3\pm0.0$&$79.6\pm0.0$&$83.6\pm0.0$&$84.7\pm0.0$\\
\multicolumn{1}{c}{}&Ll\_L21&$64.0\pm0.0$&$69.6\pm0.0$&$72.1\pm0.0$&$72.8\pm0.0$&$79.1\pm0.0$&$80.5\pm0.0$\\
\multicolumn{1}{c}{}&CIFE&$63.4\pm0.0$&$66.9\pm0.0$&$67.7\pm0.0$&$69.2\pm0.0$&$75.6\pm0.0$&$78.8\pm0.0$\\
\multicolumn{1}{c}{}&ICAP&$50.1\pm0.0$&$59.5\pm0.0$&$67.2\pm0.0$&$77.7\pm0.0$&$81.7\pm0.0$&$84.5\pm0.0$\\
\multicolumn{1}{c}{}&RFS&-&-&-&-&-&-\\
\midrule

\multirow{3}{*}{USPS}&Baseline&\multicolumn{6}{c}{97.6}\\
\multicolumn{1}{c}{}&NeuroFS&\pmb{$94.0\pm0.9$}&\pmb{$96.8\pm0.2$}&\pmb{$97.1\pm0.2$}&\pmb{$97.2\pm0.1$}&\pmb{$97.5\pm0.0$}&$97.5\pm0.1$\\
\multicolumn{1}{c}{}&LassoNet&$93.9\pm0.6$&$95.9\pm0.2$&$96.5\pm0.1$&$97.1\pm0.1$&\pmb{$97.5\pm0.1$}&\pmb{$97.6\pm0.1$}\\
\multicolumn{1}{c}{}&Fisher\_score&$82.0\pm0.0$&$91.0\pm0.0$&$94.4\pm0.0$&$96.5\pm0.0$&$97.3\pm0.0$&$97.5\pm0.0$\\
\multicolumn{1}{c}{}&Ll\_L21&$77.5\pm0.0$&$87.0\pm0.0$&$91.5\pm0.0$&$92.0\pm0.0$&$95.5\pm0.0$&$96.8\pm0.0$\\
\multicolumn{1}{c}{}&CIFE&$50.2\pm0.0$&$61.3\pm0.0$&$68.0\pm0.0$&$78.0\pm0.0$&$89.6\pm0.0$&$96.3\pm0.0$\\
\multicolumn{1}{c}{}&ICAP&$89.9\pm0.0$&$95.2\pm0.0$&$95.3\pm0.0$&$95.4\pm0.0$&$95.8\pm0.0$&$96.9\pm0.0$\\
\multicolumn{1}{c}{}&RFS&$87.4\pm0.0$&$95.3\pm0.0$&$96.5\pm0.0$&$96.7\pm0.0$&$97.2\pm0.0$&$97.3\pm0.0$\\
\midrule

\multirow{3}{*}{isolet}&Baseline&\multicolumn{6}{c}{96.0}\\
\multicolumn{1}{c}{}&NeuroFS&\pmb{$85.1\pm2.4$}&\pmb{$92.6\pm0.7$}&\pmb{$94.7\pm0.7$}&\pmb{$95.3\pm0.4$}&\pmb{$95.5\pm0.5$}&\pmb{$95.8\pm0.2$}\\
\multicolumn{1}{c}{}&LassoNet&$77.9\pm0.9$&$85.5\pm0.7$&$91.1\pm0.2$&$92.9\pm0.7$&$95.0\pm0.1$&$95.4\pm0.1$\\
\multicolumn{1}{c}{}&Fisher\_score&$57.4\pm0.0$&$67.4\pm0.0$&$76.0\pm0.0$&$79.8\pm0.0$&$83.0\pm0.0$&$89.9\pm0.0$\\
\multicolumn{1}{c}{}&Ll\_L21&$43.9\pm0.0$&$49.5\pm0.0$&$48.2\pm0.0$&$58.2\pm0.0$&$63.7\pm0.0$&$64.8\pm0.0$\\
\multicolumn{1}{c}{}&CIFE&$56.0\pm0.0$&$59.8\pm0.0$&$74.3\pm0.0$&$81.2\pm0.0$&$85.7\pm0.0$&$87.9\pm0.0$\\
\multicolumn{1}{c}{}&ICAP&$67.1\pm0.0$&$75.1\pm0.0$&$79.7\pm0.0$&$82.8\pm0.0$&$89.3\pm0.0$&$90.3\pm0.0$\\
\multicolumn{1}{c}{}&RFS&$66.5\pm0.0$&$77.3\pm0.0$&$85.1\pm0.0$&$87.8\pm0.0$&$92.5\pm0.0$&$94.9\pm0.0$\\
\midrule

\multirow{3}{*}{har}&Baseline&\multicolumn{6}{c}{95.0}\\
\multicolumn{1}{c}{}&NeuroFS&$87.5\pm1.3$&$91.4\pm0.8$&$93.1\pm0.4$&$93.8\pm0.4$&$94.8\pm0.3$&$95.4\pm0.2$\\
\multicolumn{1}{c}{}&LassoNet&\pmb{$93.0\pm0.4$}&\pmb{$94.3\pm0.3$}&\pmb{$94.7\pm0.2$}&\pmb{$95.0\pm0.3$}&\pmb{$95.6\pm0.2$}&\pmb{$95.9\pm0.0$}\\
\multicolumn{1}{c}{}&Fisher\_score&$77.1\pm0.0$&$79.8\pm0.0$&$81.7\pm0.0$&$83.8\pm0.0$&$84.4\pm0.0$&$85.8\pm0.0$\\
\multicolumn{1}{c}{}&Ll\_L21&$76.0\pm0.0$&$77.5\pm0.0$&$79.4\pm0.0$&$80.2\pm0.0$&$87.4\pm0.0$&$89.2\pm0.0$\\
\multicolumn{1}{c}{}&CIFE&$80.2\pm0.0$&$84.2\pm0.0$&$84.8\pm0.0$&$85.3\pm0.0$&$85.9\pm0.0$&$85.9\pm0.0$\\
\multicolumn{1}{c}{}&ICAP&$84.5\pm0.0$&$88.7\pm0.0$&$89.2\pm0.0$&$92.1\pm0.0$&$93.4\pm0.0$&$93.3\pm0.0$\\
\multicolumn{1}{c}{}&RFS&$84.2\pm0.0$&$88.2\pm0.0$&$88.5\pm0.0$&$89.9\pm0.0$&$91.3\pm0.0$&$92.7\pm0.0$\\
\midrule

\multirow{3}{*}{SMK}&Baseline&\multicolumn{6}{c}{86.8}\\
\multicolumn{1}{c}{}&NeuroFS&$78.9\pm1.7$&$81.6\pm1.7$&$82.6\pm2.1$&$83.2\pm1.3$&\pmb{$83.7\pm1.0$}&\pmb{$84.2\pm0.0$}\\
\multicolumn{1}{c}{}&LassoNet&$76.3\pm5.7$&$83.3\pm1.2$&$82.4\pm2.5$&$79.8\pm3.3$&$79.8\pm1.3$&$79.8\pm2.5$\\
\multicolumn{1}{c}{}&Fisher\_score&$68.4\pm0.0$&$73.7\pm0.0$&$76.3\pm0.0$&$78.9\pm0.0$&$78.9\pm0.0$&$78.9\pm0.0$\\
\multicolumn{1}{c}{}&Ll\_L21&$78.9\pm0.0$&\pmb{$84.2\pm0.0$}&\pmb{$89.5\pm0.0$}&\pmb{$84.2\pm0.0$}&$81.6\pm0.0$&$81.6\pm0.0$\\
\multicolumn{1}{c}{}&CIFE&\pmb{$81.6\pm0.0$}&$81.6\pm0.0$&$76.3\pm0.0$&$81.6\pm0.0$&$81.6\pm0.0$&$78.9\pm0.0$\\
\multicolumn{1}{c}{}&ICAP&$78.9\pm0.0$&$73.7\pm0.0$&$71.1\pm0.0$&$76.3\pm0.0$&$71.1\pm0.0$&$76.3\pm0.0$\\
\multicolumn{1}{c}{}&RFS&$78.9\pm0.0$&$76.3\pm0.0$&$76.3\pm0.0$&$71.1\pm0.0$&$71.1\pm0.0$&$71.1\pm0.0$\\
\midrule

\multirow{3}{*}{PCMAC}&Baseline&\multicolumn{6}{c}{90.2}\\
\multicolumn{1}{c}{}&NeuroFS&$82.1\pm2.6$&$80.3\pm3.2$&$83.1\pm2.5$&$82.8\pm2.3$&$83.6\pm2.7$&$82.6\pm1.7$\\
\multicolumn{1}{c}{}&LassoNet&$80.4\pm2.7$&$82.1\pm2.9$&$81.4\pm2.0$&$81.9\pm2.3$&$82.1\pm1.8$&$82.4\pm1.4$\\
\multicolumn{1}{c}{}&Fisher\_score&$81.7\pm0.0$&$86.4\pm0.0$&$85.6\pm0.0$&$84.6\pm0.0$&$84.6\pm0.0$&$84.8\pm0.0$\\
\multicolumn{1}{c}{}&Ll\_L21&$54.5\pm0.0$&$54.0\pm0.0$&$55.3\pm0.0$&$56.8\pm0.0$&$59.6\pm0.0$&$60.4\pm0.0$\\
\multicolumn{1}{c}{}&CIFE&$77.1\pm0.0$&$75.8\pm0.0$&$74.8\pm0.0$&$72.5\pm0.0$&$72.5\pm0.0$&$75.6\pm0.0$\\
\multicolumn{1}{c}{}&ICAP&\pmb{$82.8\pm0.0$}&\pmb{$87.7\pm0.0$}&\pmb{$87.9\pm0.0$}&\pmb{$87.4\pm0.0$}&\pmb{$87.9\pm0.0$}&\pmb{$88.4\pm0.0$}\\
\multicolumn{1}{c}{}&RFS&$73.8\pm0.0$&$67.6\pm0.0$&$72.2\pm0.0$&$71.0\pm0.0$&$74.3\pm0.0$&$73.5\pm0.0$\\
\midrule

    \end{tabular}}
    \end{scriptsize}
\end{table}
