# Supplementary material for: Supervised Feature Selection with Neuron Evolution in Sparse Neural Networks
Source: arXiv:2303.07200 source file (2023-03-14)
Supplement: Supplementary file 2 [file results_unsupervised.tex]

\begin{table}[!ht]
    \centering
    \caption{Unsupervised feature selection comparison (clustering accuracy (\%)) for different values of $K$ (number of selected features). Empty entries show that the corresponding experiments have exceeded the considered time limit (12 hours).} \label{tab:results_unsupervised_appendix} 
    \begin{scriptsize}
    
\scalebox{0.85}{
    \begin{tabular}{@{}c@{\hskip 0.04in}c@{\hskip 0.04in}c@{\hskip 0.04in}c@{\hskip 0.04in}c@{\hskip 0.04in}c@{\hskip 0.04in}c@{\hskip 0.04in}c@{\hskip 0.04in}}
        \toprule
         &  & \multicolumn{6}{c}{ \bt $K$}  \\
        \bt Dataset & \bt Method &\bt 25 &\bt 50 & \bt75 & \bt100 & \bt150 & \bt200  \\ \midrule

\multirow{3}{*}{coil20}&Baseline&\multicolumn{6}{c}{67.7}\\
\multicolumn{1}{c}{}&NeuroFS&$57.5\pm3.9$&$64.2\pm3.0$&\pmb{$67.3\pm2.3$}&\pmb{$68.9\pm2.2$}&$67.5\pm1.6$&$68.5\pm1.2$\\
\multicolumn{1}{c}{}&QuickSelection&\pmb{$58.2\pm0.9$}&\pmb{$65.5\pm1.8$}&$65.8\pm1.4$&$66.9\pm1.7$&\pmb{$68.8\pm1.4$}&$69.2\pm1.2$\\
\multicolumn{1}{c}{}&CAE&$53.8\pm1.7$&$59.2\pm2.2$&$60.0\pm1.4$&$58.0\pm1.9$&$59.1\pm2.5$&$59.0\pm1.2$\\
\multicolumn{1}{c}{}&MCFS&$52.0\pm0.0$&$61.4\pm0.0$&$62.7\pm0.0$&$66.7\pm0.0$&$64.7\pm0.0$&\pmb{$70.7\pm0.0$}\\
\multicolumn{1}{c}{}&Lap\_score&$47.9\pm0.0$&$56.2\pm0.0$&$58.8\pm0.0$&$55.8\pm0.0$&$55.5\pm0.0$&$58.3\pm0.0$\\
\midrule

\multirow{3}{*}{MNIST}&Baseline&\multicolumn{6}{c}{52.6}\\
\multicolumn{1}{c}{}&NeuroFS&$36.9\pm3.1$&$41.6\pm2.2$&$46.9\pm1.6$&$47.7\pm1.2$&$50.8\pm1.1$&$51.8\pm0.9$\\
\multicolumn{1}{c}{}&QuickSelection&$39.9\pm1.1$&$46.9\pm0.6$&$48.6\pm3.3$&$50.2\pm3.2$&\pmb{$52.5\pm1.4$}&\pmb{$53.5\pm0.8$}\\
\multicolumn{1}{c}{}&CAE&\pmb{$49.6\pm3.6$}&\pmb{$51.2\pm2.0$}&\pmb{$51.0\pm2.2$}&\pmb{$51.5\pm1.7$}&$52.1\pm1.4$&$52.8\pm0.8$\\
\multicolumn{1}{c}{}&MCFS&-&-&-&-&-&-\\
\multicolumn{1}{c}{}&Lap\_score&$12.4\pm0.0$&$16.3\pm0.0$&$18.0\pm0.0$&$20.7\pm0.0$&$23.6\pm0.0$&$26.7\pm0.0$\\
\midrule

\multirow{3}{*}{ \shortstack{Fashion-\\MNIST} }&Baseline&\multicolumn{6}{c}{49.9}\\
\multicolumn{1}{c}{}&NeuroFS&$44.8\pm4.3$&$45.7\pm2.9$&\pmb{$49.8\pm1.4$}&$48.8\pm1.9$&\pmb{$51.6\pm1.1$}&\pmb{$52.5\pm2.2$}\\
\multicolumn{1}{c}{}&QuickSelection&$49.7\pm1.2$&\pmb{$51.3\pm2.9$}&$49.5\pm1.7$&\pmb{$50.3\pm1.2$}&$49.7\pm2.4$&$48.8\pm3.4$\\
\multicolumn{1}{c}{}&CAE&\pmb{$50.9\pm2.2$}&$48.5\pm1.8$&$48.7\pm2.4$&$47.5\pm1.4$&$49.6\pm1.8$&$48.9\pm1.2$\\
\multicolumn{1}{c}{}&MCFS&-&-&-&-&-&-\\
\multicolumn{1}{c}{}&Lap\_score&$13.0\pm0.0$&$15.6\pm0.0$&$22.7\pm0.0$&$32.4\pm0.0$&$40.1\pm0.0$&$41.3\pm0.0$\\
\midrule

\multirow{3}{*}{USPS}&Baseline&\multicolumn{6}{c}{67.3}\\
\multicolumn{1}{c}{}&NeuroFS&$58.2\pm3.7$&\pmb{$67.3\pm3.1$}&$67.3\pm1.9$&$65.6\pm3.0$&$67.6\pm0.8$&$66.9\pm0.9$\\
\multicolumn{1}{c}{}&QuickSelection&$58.9\pm5.9$&$62.8\pm2.0$&$64.7\pm3.2$&$63.8\pm3.3$&\pmb{$69.0\pm1.1$}&$68.3\pm0.5$\\
\multicolumn{1}{c}{}&CAE&\pmb{$60.5\pm3.9$}&$64.8\pm1.8$&$64.7\pm1.0$&$64.6\pm1.4$&$64.5\pm2.4$&$65.6\pm0.9$\\
\multicolumn{1}{c}{}&MCFS&$50.8\pm0.0$&$62.9\pm0.0$&\pmb{$68.9\pm0.0$}&\pmb{$69.5\pm0.0$}&\pmb{$69.0\pm0.0$}&\pmb{$68.9\pm0.0$}\\
\multicolumn{1}{c}{}&Lap\_score&$35.1\pm0.0$&$40.1\pm0.0$&$52.1\pm0.0$&$55.9\pm0.0$&$59.9\pm0.0$&$65.1\pm0.0$\\
\midrule

\multirow{3}{*}{isolet}&Baseline&\multicolumn{6}{c}{57.8}\\
\multicolumn{1}{c}{}&NeuroFS&$37.9\pm2.8$&$44.9\pm3.0$&\pmb{$48.8\pm2.8$}&\pmb{$49.4\pm2.4$}&\pmb{$53.6\pm2.4$}&\pmb{$55.7\pm1.7$}\\
\multicolumn{1}{c}{}&QuickSelection&$31.7\pm3.0$&$37.7\pm2.4$&$39.8\pm1.9$&$42.5\pm2.8$&$44.0\pm2.0$&$44.6\pm2.8$\\
\multicolumn{1}{c}{}&CAE&$30.7\pm1.4$&$38.1\pm3.9$&$39.4\pm2.7$&$40.0\pm2.6$&$38.7\pm1.1$&$38.6\pm1.5$\\
\multicolumn{1}{c}{}&MCFS&\pmb{$42.1\pm0.0$}&\pmb{$45.4\pm0.0$}&$42.2\pm0.0$&$48.3\pm0.0$&$47.4\pm0.0$&$47.1\pm0.0$\\
\multicolumn{1}{c}{}&Lap\_score&$33.6\pm0.0$&$39.4\pm0.0$&$42.2\pm0.0$&$45.6\pm0.0$&$47.0\pm0.0$&$45.5\pm0.0$\\
\midrule

\multirow{3}{*}{har}&Baseline&\multicolumn{6}{c}{56.6}\\
\multicolumn{1}{c}{}&NeuroFS&$53.9\pm0.7$&$54.4\pm0.8$&$54.8\pm1.4$&$55.1\pm0.9$&$54.9\pm1.2$&$54.9\pm1.0$\\
\multicolumn{1}{c}{}&QuickSelection&$54.9\pm0.5$&$55.1\pm2.0$&$56.3\pm0.9$&$56.2\pm0.6$&$56.3\pm0.3$&$56.1\pm0.4$\\
\multicolumn{1}{c}{}&CAE&$53.6\pm4.3$&$53.2\pm2.5$&$54.2\pm1.2$&$54.5\pm0.8$&$54.6\pm0.4$&$54.5\pm0.7$\\
\multicolumn{1}{c}{}&MCFS&$45.3\pm0.0$&$57.3\pm0.0$&$56.8\pm0.0$&\pmb{$58.7\pm0.0$}&\pmb{$57.6\pm0.0$}&\pmb{$56.8\pm0.0$}\\
\multicolumn{1}{c}{}&Lap\_score&\pmb{$61.8\pm0.0$}&\pmb{$61.3\pm0.0$}&\pmb{$61.3\pm0.0$}&$56.4\pm0.0$&$56.1\pm0.0$&$56.2\pm0.0$\\
\midrule

\multirow{3}{*}{SMK}&Baseline&\multicolumn{6}{c}{53.0}\\
\multicolumn{1}{c}{}&NeuroFS&$53.7\pm2.6$&$52.3\pm1.9$&$52.6\pm2.6$&$53.0\pm2.3$&$52.1\pm2.3$&$51.8\pm1.8$\\
\multicolumn{1}{c}{}&QuickSelection&$52.6\pm1.3$&$53.8\pm1.0$&$53.4\pm1.9$&$52.5\pm2.0$&$52.0\pm1.3$&$52.3\pm2.0$\\
\multicolumn{1}{c}{}&CAE&$51.2\pm1.1$&$51.5\pm0.8$&$51.6\pm1.8$&$52.8\pm2.7$&$52.5\pm1.8$&$51.7\pm1.2$\\
\multicolumn{1}{c}{}&MCFS&\pmb{$54.9\pm0.0$}&\pmb{$54.2\pm0.0$}&$51.3\pm0.0$&$50.9\pm0.0$&$52.9\pm0.0$&$55.3\pm0.0$\\
\multicolumn{1}{c}{}&Lap\_score&$50.3\pm0.0$&$54.0\pm0.0$&\pmb{$56.9\pm0.0$}&\pmb{$53.7\pm0.0$}&\pmb{$55.6\pm0.0$}&\pmb{$56.2\pm0.0$}\\
\midrule

\multirow{3}{*}{PCMAC}&Baseline&\multicolumn{6}{c}{50.9}\\
\multicolumn{1}{c}{}&NeuroFS&$51.0\pm0.0$&$50.9\pm0.0$&\pmb{$50.9\pm0.1$}&$50.9\pm0.0$&$50.9\pm0.1$&$50.9\pm0.0$\\
\multicolumn{1}{c}{}&QuickSelection&$50.9\pm0.1$&$50.9\pm0.2$&\pmb{$50.9\pm0.1$}&\pmb{$51.0\pm0.0$}&\pmb{$51.0\pm0.0$}&\pmb{$51.0\pm0.0$}\\
\multicolumn{1}{c}{}&CAE&$50.6\pm0.1$&$50.6\pm0.1$&$50.6\pm0.1$&$50.6\pm0.1$&$50.6\pm0.1$&$50.7\pm0.2$\\
\multicolumn{1}{c}{}&MCFS&\pmb{$51.2\pm0.0$}&\pmb{$51.2\pm0.0$}&$50.8\pm0.0$&$50.8\pm0.0$&\pmb{$51.0\pm0.0$}&\pmb{$51.0\pm0.0$}\\
\multicolumn{1}{c}{}&Lap\_score&$50.6\pm0.0$&$50.6\pm0.0$&$50.6\pm0.0$&$50.6\pm0.0$&$50.4\pm0.0$&$50.3\pm0.0$\\
\midrule

    \end{tabular}}
    \end{scriptsize}
\end{table}
