# Supplementary material for: Supervised Feature Selection with Neuron Evolution in Sparse Neural Networks
Source: arXiv:2303.07200 source file (2023-03-14)
Supplement: Supplementary file 3 [file table_gradient_random.tex]

\begin{table}[ht]
    \centering
    \caption{Ablation study: gradient vs. random policy (for weight and neuron selection) comparison (classification accuracy (\%)).} \label{tab:results_ablation_gradient} 
    \begin{scriptsize}
    
\scalebox{0.75}{
    \begin{tabular}{@{}c@{\hskip 0.02in}c@{\hskip 0.04in}c@{\hskip 0.04in}c@{\hskip 0.04in}c@{\hskip 0.07in}c@{\hskip 0.04in}c@{\hskip 0.04in}c@{\hskip 0.07in}}
        \toprule
         &  & \multicolumn{6}{c}{ \bt $K$}  \\
        \bt Dataset & \bt Method &\bt 25 &\bt 50 & \bt75 & \bt100 & \bt150 & \bt200  \\ \midrule

\multicolumn{1}{c}{coil20}&NeuroFS&\pmb{$96.2\pm0.8$}&\pmb{$98.8\pm0.2$}&\pmb{$98.9\pm0.3$}&\pmb{$99.2\pm0.5$}&\pmb{$100.0\pm0.0$}&\pmb{$99.9\pm0.1$}\\
\multicolumn{1}{c}{}&NeuroFS[w/oGradient]&$80.7\pm1.5$&$88.4\pm2.5$&$92.0\pm1.4$&$92.9\pm0.7$&$94.3\pm2.0$&$96.4\pm2.2$\\
\midrule

\multicolumn{1}{c}{MNIST}&NeuroFS&$87.9\pm1.8$&$95.3\pm0.4$&$96.8\pm0.2$&$97.3\pm0.2$&$97.7\pm0.1$&$97.9\pm0.1$\\
\multicolumn{1}{c}{}&NeuroFS[w/oGradient]&\pmb{$90.8\pm0.5$}&\pmb{$96.3\pm0.3$}&\pmb{$97.2\pm0.2$}&\pmb{$97.7\pm0.1$}&\pmb{$98.0\pm0.1$}&\pmb{$98.1\pm0.0$}\\
\midrule

\multicolumn{1}{c}{Fashion-MNIST}&NeuroFS&\pmb{$79.4\pm1.0$}&$83.8\pm0.6$&$85.7\pm0.3$&\pmb{$86.6\pm0.2$}&$87.2\pm0.2$&$87.5\pm0.2$\\
\multicolumn{1}{c}{}&NeuroFS[w/oGradient]&$78.7\pm1.0$&\pmb{$84.0\pm0.3$}&\pmb{$85.9\pm0.4$}&$86.5\pm0.3$&\pmb{$87.5\pm0.1$}&\pmb{$88.0\pm0.1$}\\
\midrule

\multicolumn{1}{c}{USPS}&NeuroFS&$94.0\pm0.9$&\pmb{$96.8\pm0.2$}&\pmb{$97.1\pm0.2$}&$97.2\pm0.1$&\pmb{$97.5\pm0.0$}&$97.5\pm0.1$\\
\multicolumn{1}{c}{}&NeuroFS[w/oGradient]&\pmb{$94.3\pm0.7$}&$96.2\pm0.3$&$97.0\pm0.2$&\pmb{$97.3\pm0.1$}&\pmb{$97.5\pm0.1$}&\pmb{$97.6\pm0.0$}\\
\midrule

\multicolumn{1}{c}{isolet}&NeuroFS&\pmb{$85.1\pm2.4$}&\pmb{$92.6\pm0.7$}&\pmb{$94.7\pm0.7$}&\pmb{$95.3\pm0.4$}&$95.5\pm0.5$&\pmb{$95.8\pm0.2$}\\
\multicolumn{1}{c}{}&NeuroFS[w/oGradient]&$83.3\pm0.9$&\pmb{$92.6\pm1.2$}&$93.9\pm0.2$&$94.8\pm0.4$&\pmb{$95.6\pm0.4$}&$95.6\pm0.3$\\
\midrule

\multicolumn{1}{c}{har}&NeuroFS&\pmb{$87.5\pm1.3$}&$91.4\pm0.8$&$93.1\pm0.4$&$93.8\pm0.4$&$94.8\pm0.3$&\pmb{$95.4\pm0.2$}\\
\multicolumn{1}{c}{}&NeuroFS[w/oGradient]&$86.3\pm0.5$&\pmb{$91.7\pm0.9$}&\pmb{$93.9\pm0.4$}&\pmb{$94.4\pm0.3$}&\pmb{$94.9\pm0.3$}&$95.1\pm0.2$\\
\midrule

\multicolumn{1}{c}{SMK}&NeuroFS&$78.9\pm1.7$&$81.6\pm1.7$&$82.6\pm2.1$&\pmb{$83.2\pm1.3$}&\pmb{$83.7\pm1.0$}&\pmb{$84.2\pm0.0$}\\
\multicolumn{1}{c}{}&NeuroFS[w/oGradient]&\pmb{$85.2\pm2.1$}&\pmb{$84.2\pm2.9$}&\pmb{$85.3\pm2.7$}&$80.5\pm2.1$&$83.1\pm2.7$&$82.1\pm2.0$\\
\midrule

\multicolumn{1}{c}{PCMAC}&NeuroFS&$82.1\pm2.6$&$80.3\pm3.2$&$83.1\pm2.5$&$82.8\pm2.3$&$83.6\pm2.7$&$82.6\pm1.7$\\
\multicolumn{1}{c}{}&NeuroFS[w/oGradient]&\pmb{$84.0\pm0.6$}&\pmb{$83.8\pm1.0$}&\pmb{$83.9\pm2.2$}&\pmb{$84.5\pm1.1$}&\pmb{$84.7\pm1.4$}&\pmb{$84.7\pm0.6$}\\
\midrule

    \end{tabular}}
    \end{scriptsize}
\end{table}
