# Supplementary material for: Supervised Feature Selection with Neuron Evolution in Sparse Neural Networks
Source: arXiv:2303.07200 source file (2023-03-14)
Supplement: Supplementary file 4 [file alg_ctre_seq.tex]

\begin{figure}[!t]
\vskip -0.4 in
\begin{minipage}[t]{0.49\textwidth}
\begin{algorithm}[H]
    \caption{CTRE\textsubscript{seq}}
    \label{alg:CTRE_seq}
     \scriptsize
    \begin{algorithmic}[1]
        \State \textbf{Input}: Dataset $\displaystyle \sX$, sparsity hyperparameter $\varepsilon$, drop fraction $\zeta$, early stop epoch $e_{early\;stop}$
        \State Initialize the network with sparsity determined by $\varepsilon$,  $flag_{random\;search} = False$
        \For{\texttt{$i \in \{1,\dots, \#epochs\}$}}
            \State perform standard feed-forward and back-propagation
            \For{\texttt{$l \in \{1,\dots, H\}$}}
                \State Remove $\zeta N^l$ of the weights with smallest magnitude.
                \If{$flag_{random\;search}$}
                    \State Add $\zeta N^l$ connections randomly
                \Else
                    \State Compute Similarity matrix $\displaystyle \mSim^{l}$ according to Equation \ref{eq:cosine_similarity}
                    \State \multiline{%
                    Add $\zeta N^l$ connections with the highest similarity value in $\displaystyle \mSim^{l}$}
                \EndIf
            \EndFor
        %    \State \texttt{${{s}_{i}}=\sum\limits_{j=1}^{n^h}{|{{W}^{1}_{ij}}}|$
        %    }
        \If{Accuracy on validation set does not improve in $e_{early\;stop}$}
            \State Set $flag_{random\;search} = True$
        \EndIf
        \EndFor
        \end{algorithmic}

    \end{algorithm}

\end{minipage}
\hfill
\begin{minipage}[t]{0.49\textwidth}

\begin{algorithm}[H]
    \caption{CTRE\textsubscript{sim }}
    \label{alg:CTRE_sim}
     \scriptsize
    \begin{algorithmic}[1]
        \State \textbf{Input}: Dataset $\displaystyle \sX$, sparsity hyperparameter $\varepsilon$, drop fraction $\zeta$
        \State Initialize the network with sparsity determined by $\varepsilon$
        \For{\texttt{$i \in \{1,\dots, \#epochs\}$}}
            \State perform standard feed-forward and back-propagation
            \For{\texttt{$l \in \{1,\dots, H\}$}}
                \State Remove $\zeta N^l$ of the weights with smallest magnitude.
                \State Compute Similarity matrix $\displaystyle \mSim^{l}$ according to Equation \ref{eq:cosine_similarity}
                \State \multiline{%
                $C_{sim}$ = Set of $\zeta N^l$ connections with the highest similarity value in $\displaystyle \mSim^{l}$}
                \For{each \texttt{$c \in C_{sim}$}} 
                    \If{$c$ was removed in the last weight removal step}
                        \State Add a random connection to the network
                    \Else
                        \State Add connection $c$ to the network
                    \EndIf 
                \EndFor
            \EndFor
        %    \State \texttt{${{s}_{i}}=\sum\limits_{j=1}^{n^h}{|{{W}^{1}_{ij}}}|$
        %    }

        %\EndIf
        \EndFor
        \end{algorithmic}
 
    \end{algorithm}

\end{minipage}
\vskip -0.2 in
\end{figure}

\begin{comment}

\begin{algorithm}[!b]
    \caption{CTRE\textsubscript{seq}}
    \label{alg:CTRE_seq}
    \begin{algorithmic}[1]
        \State \textbf{Input}: Dataset $\displaystyle \sX$, sparsity hyperparameter $\varepsilon$, drop fraction $\zeta$, early stop epoch $e_{early\;stop}$
        \State Initialize the network with sparsity determined by $\varepsilon$,  $flag_{random\;search} = False$
        \For{\texttt{$i \in \{1,\dots, \#epochs\}$}}
            \State perform standard feed-forward and back-propagation
            \For{\texttt{$l \in \{1,\dots, \#layers\}$}}
                \State Remove $\zeta$ fraction of the weights with smallest magnitude.
                \If{$flag_{random\;search}$}
                    \State Add connections randomly, the same amount as removed as removed previously
                \Else
                    \State Compute Similarity matrix $\displaystyle \mSim^{l}$ according to Equation \ref{eq:cosine_similarity}
                    \State \multiline{%
                    Add connections with the highest similarity value in $\displaystyle \mSim^{l}$, the same amount as removed previously}
                \EndIf
            \EndFor
        %    \State \texttt{${{s}_{i}}=\sum\limits_{j=1}^{n^h}{|{{W}^{1}_{ij}}}|$
        %    }
        \If{Accuracy on validation set does not improve in $e_{early\;stop}$}
            \State Set $flag_{random\;search} = True$
        \EndIf
        \EndFor
        \end{algorithmic}
 
    \end{algorithm}
    
\end{comment}
